# Supplementary material for: An analysis of document graph construction methods for AMR summarization
Source: arXiv:2111.13993 source file (2021-11-27)
Supplement: Supplementary file 1 [file app_adjudication.tex]

\section{Annotation Adjudication Instructions}
\label{app:adjudication}

After completing the initial round of annotations,
annotators were given the following adjudication instructions:

\paragraph{Instructions for AMR adjudication}
Hello, all! It is about midway through the week, but I thought I'd send out some additional guidelines to give some more context on what the overall goal of these annotations are, just in case there are any lingering confusions.

\paragraph{What are these annotations for?}
The point of these annotations is to identify which document nodes correspond \textit{exactly} (or, with an abstractive tag, \textit{roughly}) with a summary node. The ultimate goal is that, if we took the set of all document nodes that were labeled with the same summary node and merged them all, we'd end up with one document node that represented that entity across sentences.\\

What do I mean by this? Let's say you have two sentences in your document that refer to Roscoe: ``Roscoe is a brown dog. Roscoe likes peanut butter." Our nodes here will probably be something like:\\

\begin{figure}[H]
    \centering
        \resizebox{0.5\textwidth}{!}{
    \includegraphics[width=5in]{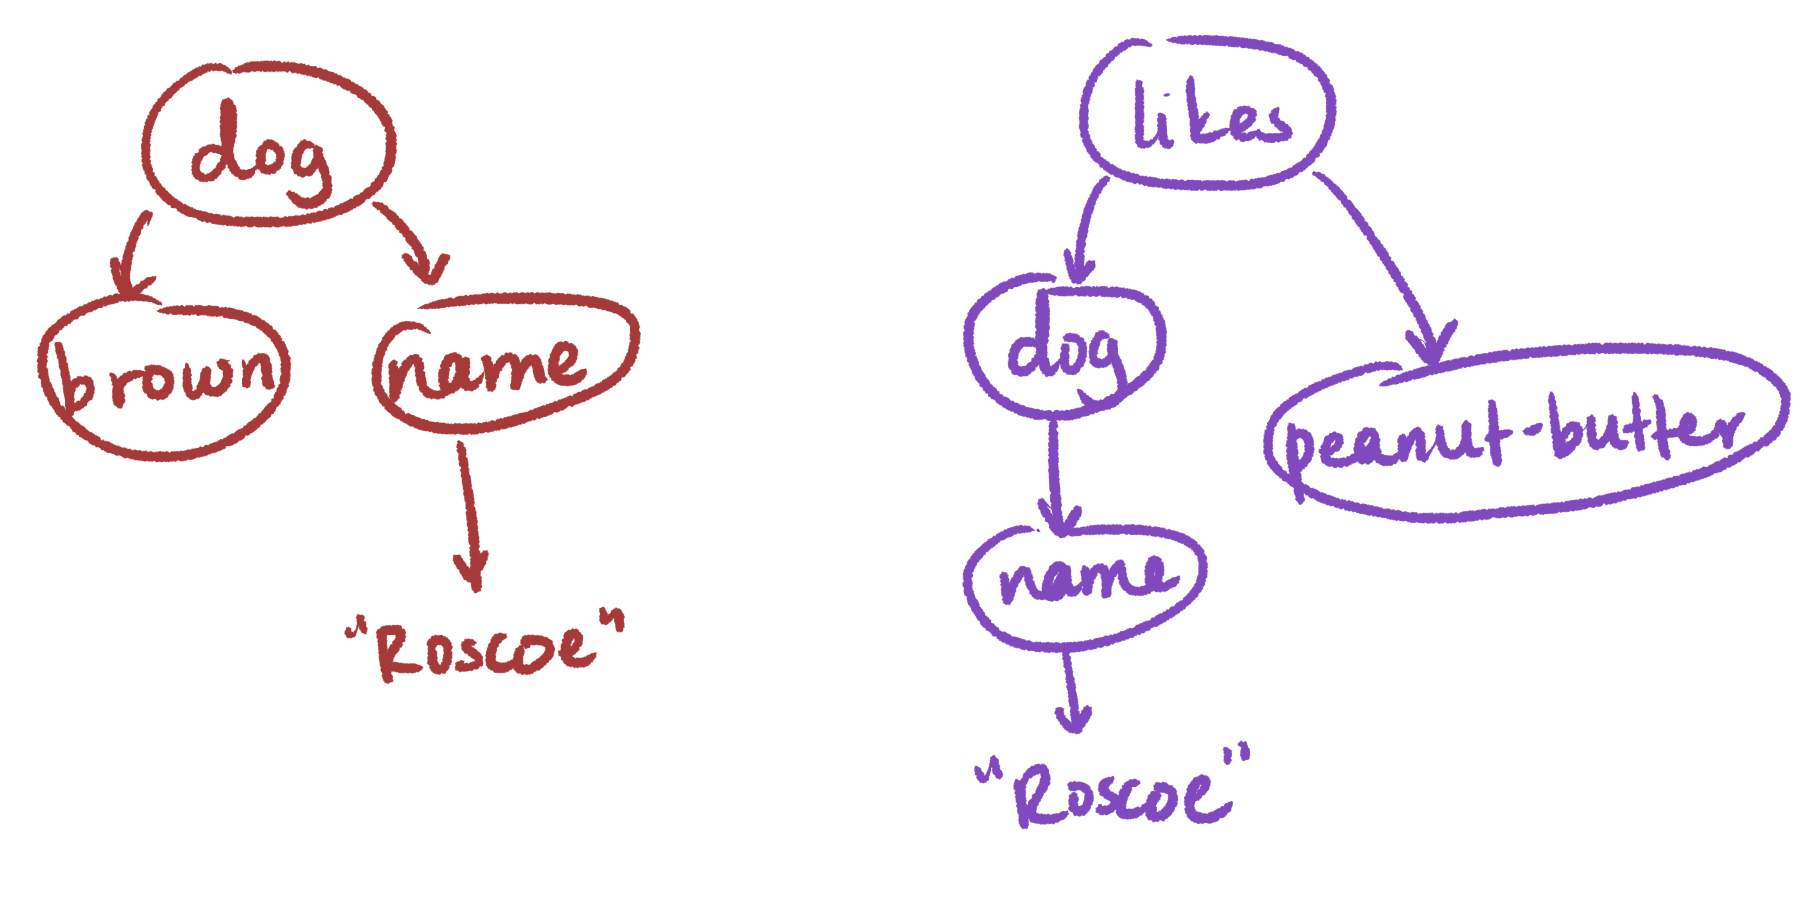}}
    \label{fig:roscoe}
\end{figure}

To keep things simple, let's say our summary is just ``Roscoe is a dog".

\begin{figure}[H]
    \centering
        \resizebox{0.5\textwidth}{!}{
    \includegraphics[width=5in]{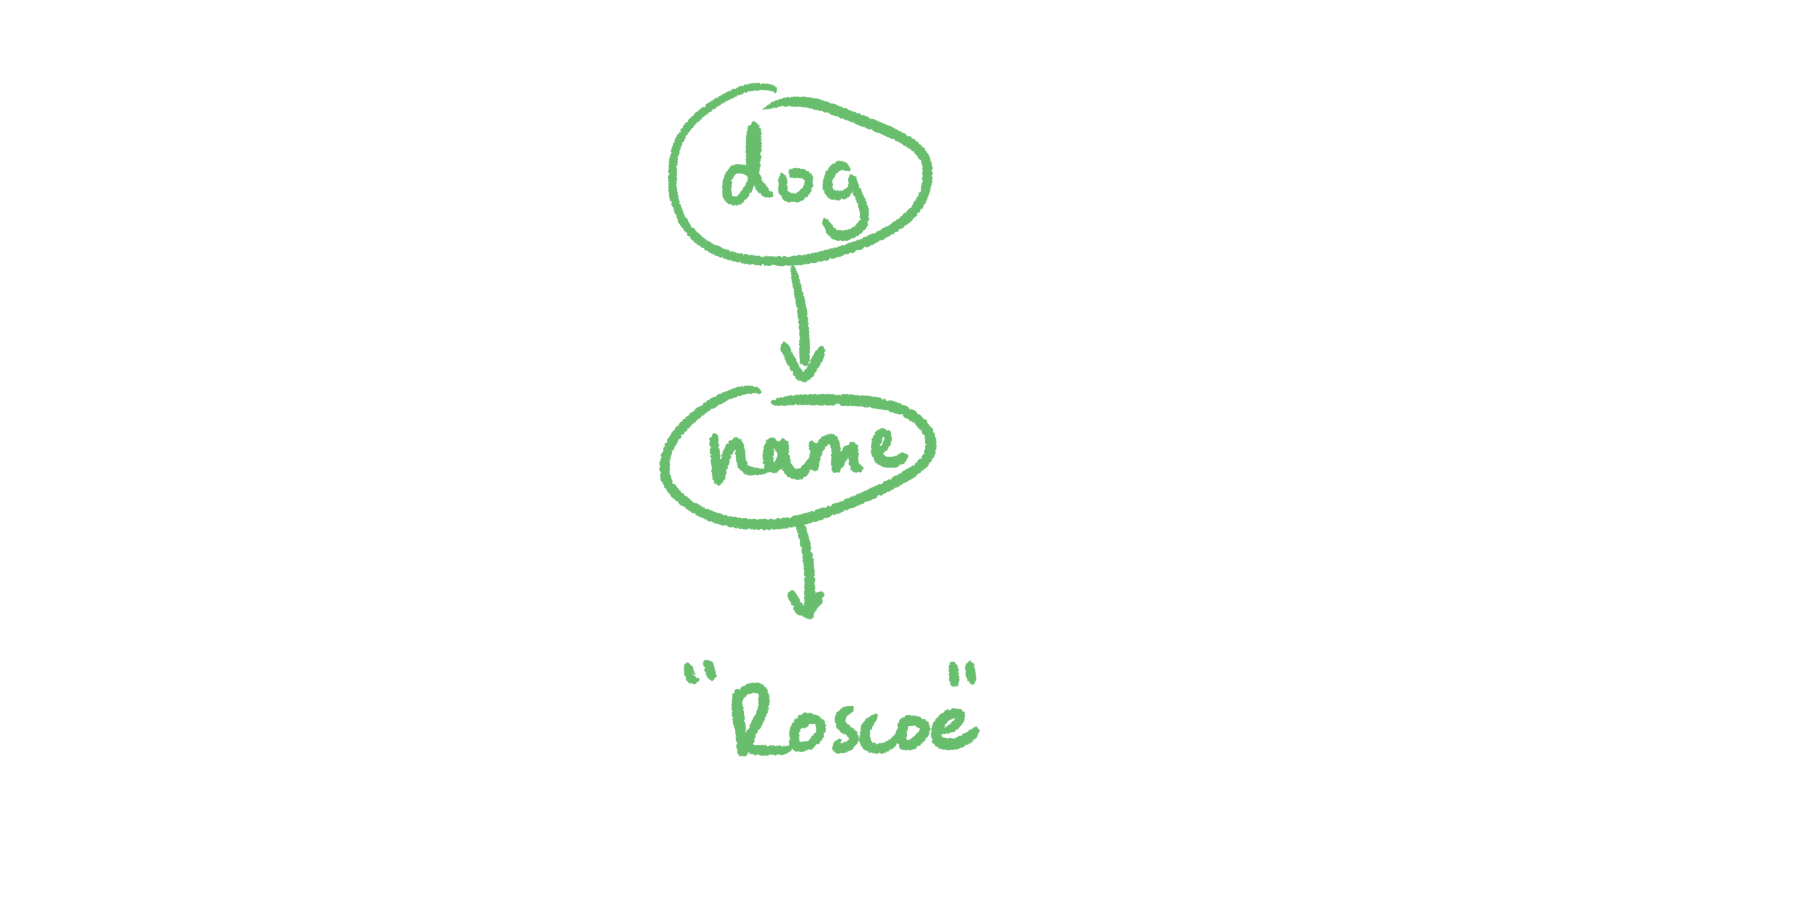}}
    \label{fig:roscoe-summary}
\end{figure}

In this case we'd want to align the ``dog" nodes in the first and second sentences with the ``dog" node in the summary, and the ``name" nodes in the first and second sentences with the ``name" node in the summary. Going back the other way, this means we've identified both ``dog" nodes as having the same summary node match, as well as both the ``name" nodes. So if we were to merge those sets of nodes in the original graph, we'd get:

\begin{figure}[H]
    \centering
        \resizebox{0.5\textwidth}{!}{
    \includegraphics[width=5in]{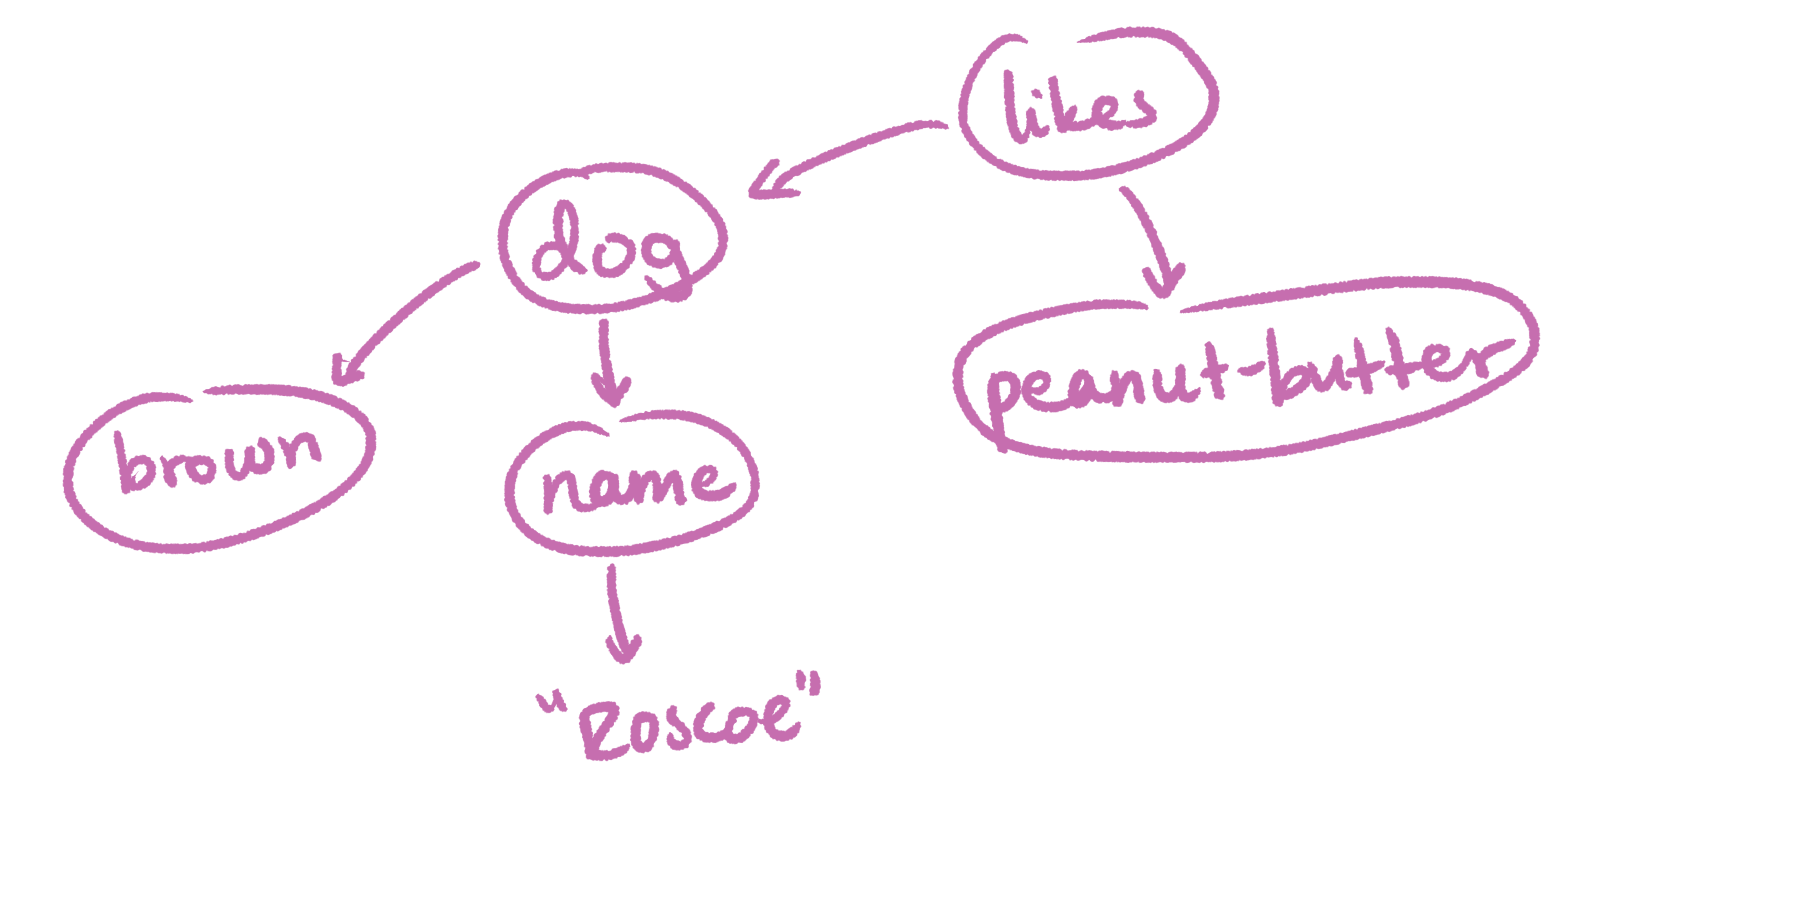}
    }
    \label{fig:roscoe-merged}
\end{figure}

This is the kind of graph we want to be able to generate in the end - all nodes (and only nodes) that refer to the same entity are merged into a single node with that identity. Ultimately, the goal is to be able to do node-level classification over this graph to extract a summary subgraph that approximates the (similarly merged) graph for the summary. Basically, whatever matching we do from document to summary, we want to be able to substitute the the summary node(s) we matched any document node to in place of that document node without substantially changing the meaning of that part of the sentence.

\paragraph{So what does this mean for annotation?}
Of course the real data is nowhere near as clean as the above example, as I am sure you are all very well aware by now. So here are a few cases where things might get confusing:

\paragraph{Do you match the whole phrase or just the base node?}
For example, if we had an ``orange cat" in the summary and we just have a ``cat" in the document, does ``cat" get matched to both orange and cat? The short answer: no, just match ``cat" with ``cat".\\

The longer answer: sometimes it's a bit more confusing than this. For example, if you have ``annotators' union representative" in the summary, and just ``spokesperson" in the document, it's a bit harder to figure out what to match it to, since the information of the person's role is implicit. But here, again, the node(s) for ``spokesperson" should only be matched to the corresponding node(s) in ``representative", since that's the actual entity that is the same.

\paragraph{Something is broken up into multiple parts.}
Let's say your summary sentence is \green{An annotators' union representative criticized the lack of pet pictures in the annotation guidelines.} and the document sentence you're looking at is \blue{The annotators' union officially expresses its disappointment in the lack of dog and cat pictures in the released annotation guidelines despite all the pet-related examples, a spokesperson said earlier today.} (Sorry about that.)\\

All seems to be going well until you get to \blue{expresses its disappointment} - suddenly you realize that the single node \green{criticize-01} in the summary seems to be broken up into two nodes here, \blue{express-01} and \blue{disappointment}. So what gets matched?\\

In this case, keeping in mind that we want to be able to swap in our match, I would say both \blue{express-01} and \blue{disappointment} get matched to \green{criticize-01} - in the graph, those two nodes together do basically the same thing a single \blue{criticize-01} node would. But neither node plays exactly the same role that \blue{criticize-01} does, so both would be marked with \texttt{abs}.\\

However, it really depends on the situation, so in general, just use your best judgement (sorry!). But hopefully the example is at least a bit helpful.

\paragraph{Abstract vs concrete instance mentions}
Let's expand our example from above: the summary is \green{An annotators' union representative criticized the lack of pet pictures in the annotation guidelines.} The document is \blue{The annotators' union officially expresses its disappointment in the lack of dog and cat pictures in the released annotation guidelines despite all the pet-related examples, a spokesperson said earlier today. It is common knowledge in the annotation trade that pet pictures make any annotation guidelines better.}\\

Well, we're finally past the first document sentence (phew). But here in the second sentence things get tricky. You could make a reasonable argument that the ``annotate" in ``annotation trade" is the same ``annotate" in ``annotators' union", sure. But how about ``annotation guidelines"? There's an \green{annotation guidelines} in the summary, and an \blue{annotation guidelines} in the document - but the former is pretty clearly referring to a \textit{specific instance} of annotation guidelines, while the latter is talking about annotation guidelines in general. But the class of annotation guidelines in general includes the particular annotation guidelines the summary is talking about. So does it get matched?\\

Here the answer is no. The abstract class of all of a certain kind of thing is separate from any specific instance of that thing, so there's no match. (If it helps to think about it this way, we wouldn't want to merge/identify these nodes in the graph because then the second document sentence would be saying ``it's common knowledge in the annotation trade that pet pictures make 
%CK: redacted FT's name of anonymity 
%Fei-Tzin's 
AMR annotation guidelines better", which is nonsensical.)
