# Supplementary material for: An analysis of document graph construction methods for AMR summarization
Source: arXiv:2111.13993 source file (2021-11-27)
Supplement: Supplementary file 4 [file app_alignments.tex]

\section{Document-summary node alignments}
\label{app:alignments}

We provide an example of the node alignments between two document sentences and a summary sentence in \autoref{fig:alignments}.
