# Supplementary material for: An analysis of document graph construction methods for AMR summarization
Source: arXiv:2111.13993 source file (2021-11-27)
Supplement: Supplementary file 6 [file app_annotations.tex]

\section{Annotation guidelines and interface}
\label{app:annotations}
Annotators were given the following guidelines:

\definecolor{grayish}{HTML}{8080a0}
\definecolor{greenish}{HTML}{20d040}
\definecolor{blueish}{HTML}{40a0f0}
\definecolor{purplish}{HTML}{f040a0}
\definecolor{refcolor}{HTML}{2020a0}

\newcommand{\green}[1]{\textbf{\textcolor{greenish}{#1}}}
\newcommand{\blue}[1]{\textbf{\textcolor{blueish}{#1}}}
\newcommand{\purple}[1]{\textcolor{purplish}{#1}}
\paragraph{Instructions for AMR alignment}
First of all, thanks so much for agreeing to do these annotations! I can't offer real cookies but you have all the virtual cookies my gratitude can buy. By all means, go ahead and turn off your ad tracker and click around on Facebook. Treat yourself.\\

This document contains four sections: (1) a task overview, with a toy example illustrating the annotation data format; (2) a description of the files you are provided; (3) the annotation instructions themselves; and (4) annotation tips and tricks. If the task makes sense to you and you think you have a good handle on how to do it, you may want to skip or skim sections 1 and 4. But please read sections 2 and 3 carefully, as this is where the actual instructions are.\\

There are also an appendix you can optionally use as reference that contains a more realistic worked example than the toy example in Section 4.

\paragraph{Overview and small example}
In this annotation task, you will be asked to perform \purple{coreference between entities} in a document and its summary. More specifically, you will be asked to align nodes of a semantic graph representing part of a news article to nodes of the semantic graphs that represent its summary. Concretely, you'll be aligning nodes of the AMR graphs for document sentences to the nodes of the AMR graph for summary sentences that \purple{refer to the same thing}. In these instructions, we will refer to these nodes as ``entities"; however, keep in mind that said ``entities" may be verbs or other relations as well as nouns.\\

If you aren't familiar with AMR, the short explanation is that it's a type of semantic graph where concepts are represented by nodes in the graph, and the edges represent the relations between the concepts that are present in the text. One thing to note is that the nodes in AMR may not line up exactly with the entities that are explicitly present in the text, but it isn't too hard to figure out what each node refers to if you look at the nodes around it.\\

Sound too abstract? Let's do a toy example.\\

We'll consider the following document: \blue{Roscoe is Kathy's dog. Roscoe likes to jump. He and Pippin the cat are playing tag.} And here's our summary: \green{Kathy's dog Roscoe likes to jump. He is playing with a cat.}\\

So the AMR graphs for the document and summary sentences will look something like this:

\begin{figure}[H]
    \centering
    \resizebox{0.5\textwidth}{!}{
    \includegraphics{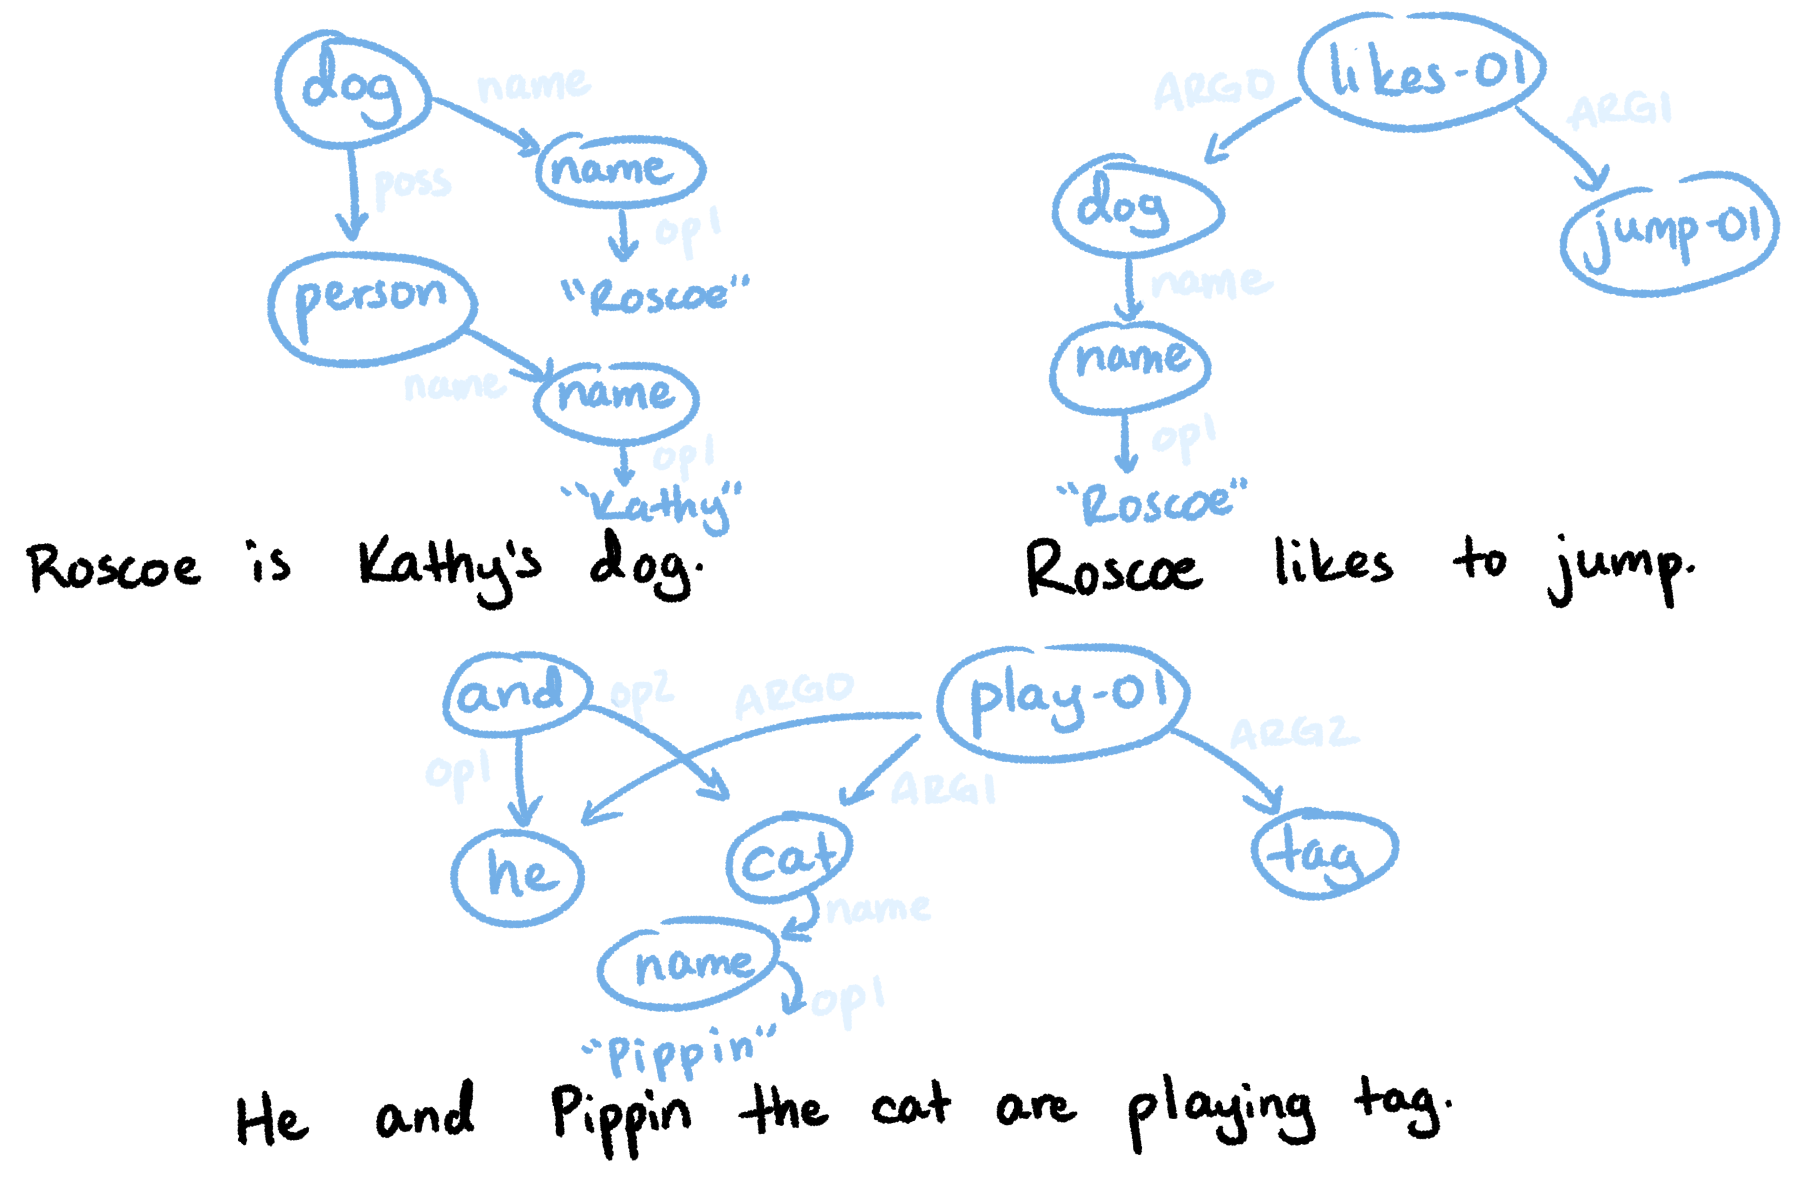}}
    \label{fig:sample-doc}
\end{figure}

\begin{figure}[H]
    \centering
        \resizebox{0.5\textwidth}{!}{
    \includegraphics{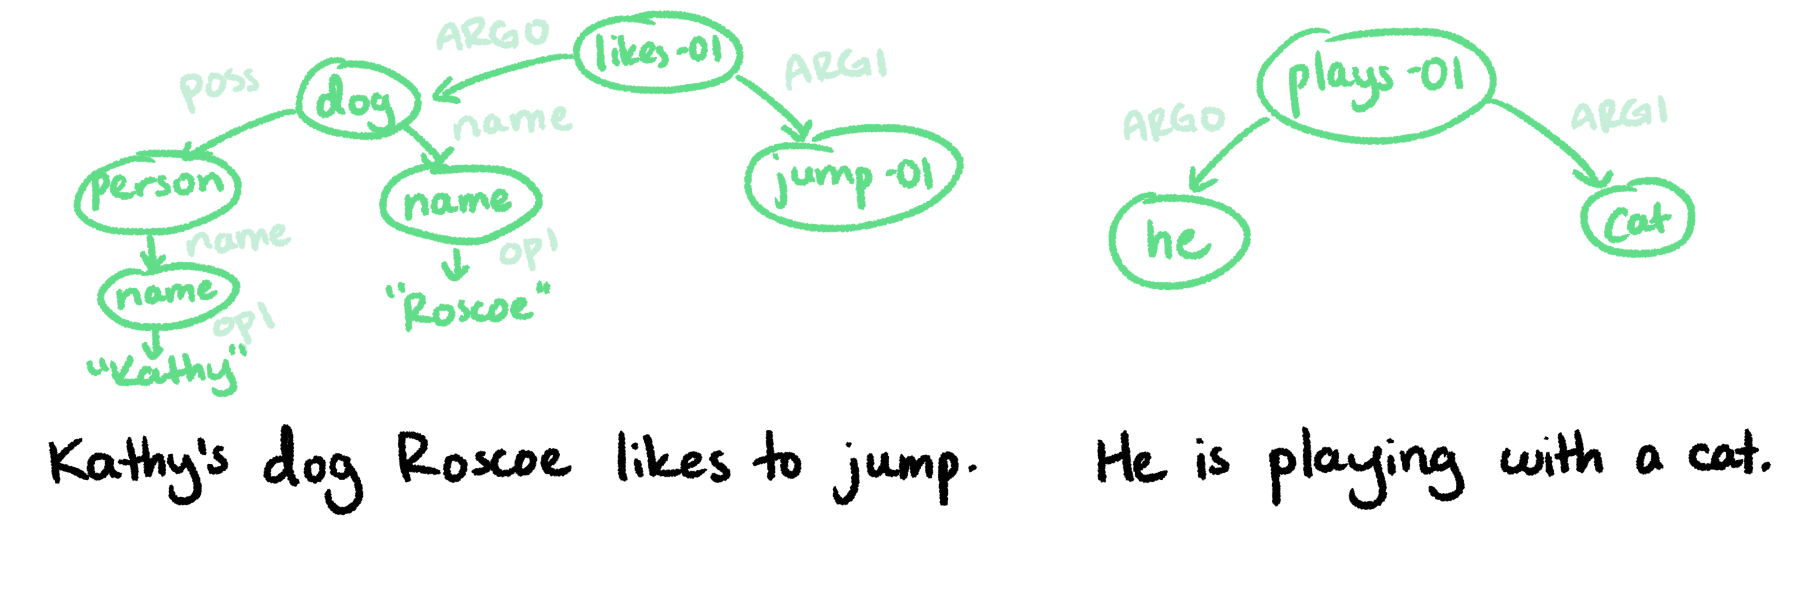}}
    \label{fig:sample-summary}
\end{figure}

So, great, that's a bunch of graphs. Don't worry too much if you find these hard to read; we actually don't need the graph structure for much. For the purposes of this task, all we truly want to do is match nodes to nodes.

So when we convert the AMR graphs into the format for annotation, for each sentence, we'll just end up with a list of nodes, like so (although in our files we'll always list the summary first):

\begin{figure}[H]
    \centering     
    \resizebox{0.5\textwidth}{!}{
    \includegraphics[height=8in]{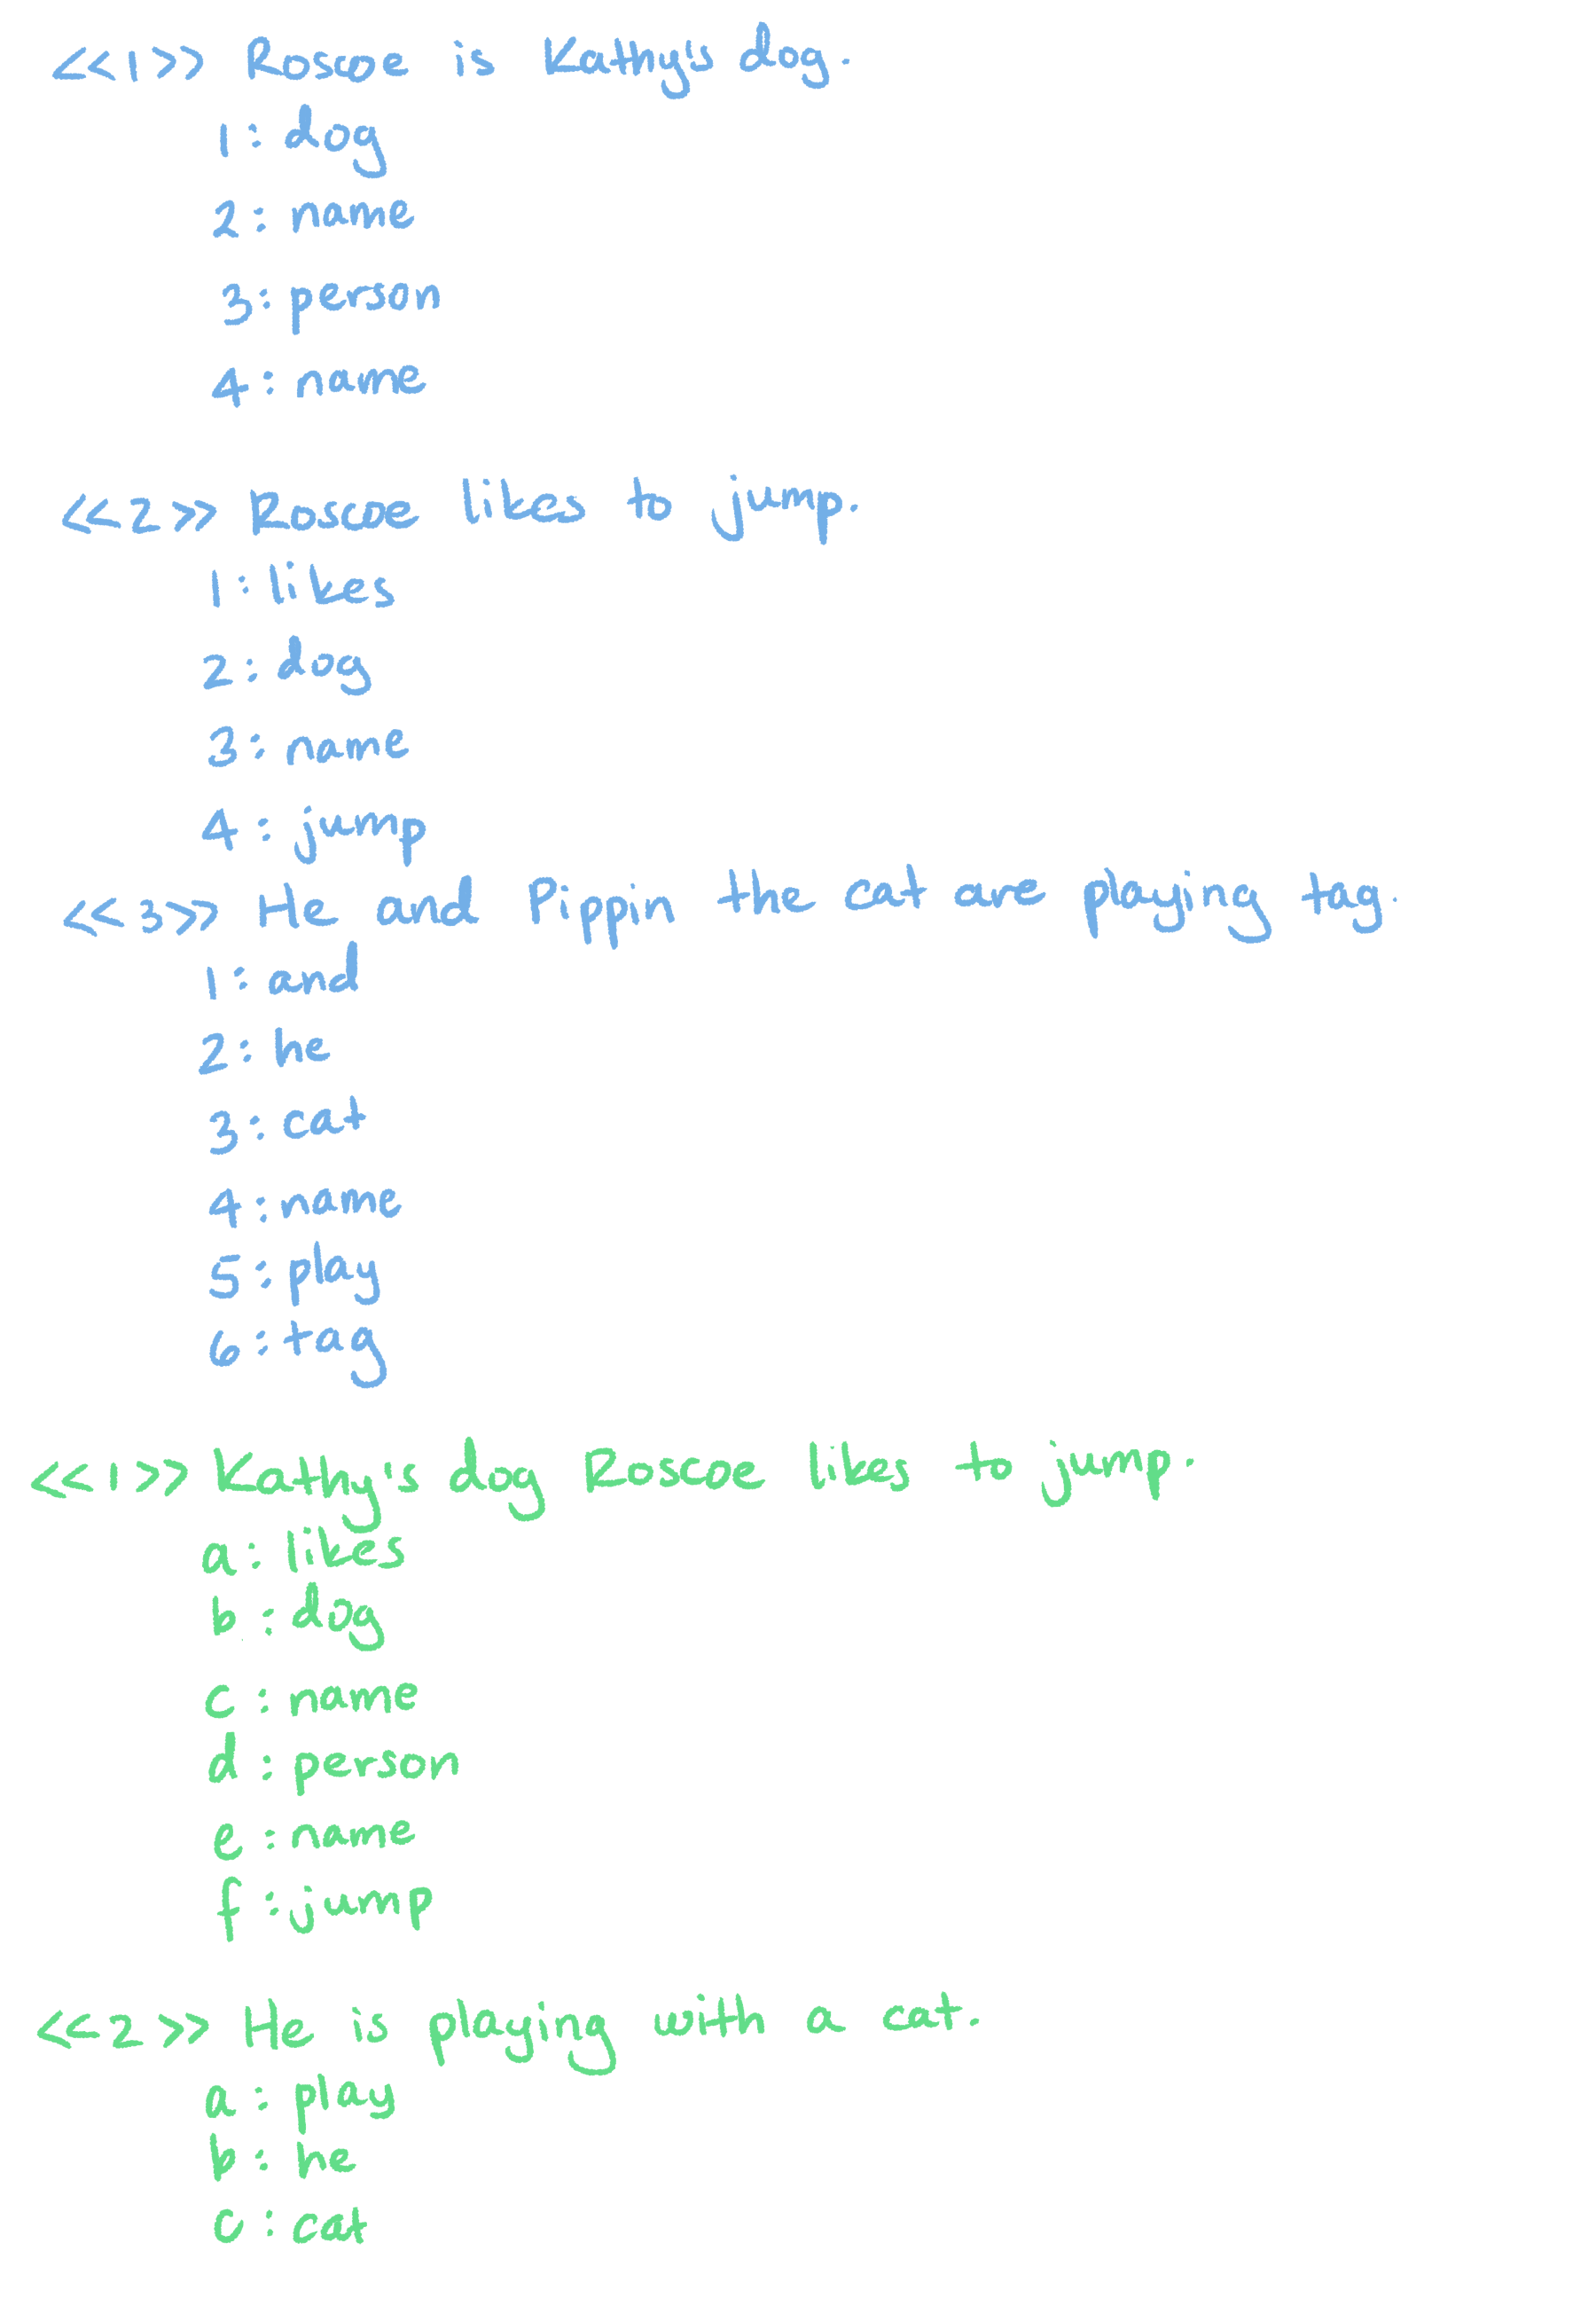}}
    \label{fig:sample-nodes}
\end{figure}

When we annotate, what we want to do is mark each document node with \purple{all} the summary nodes that it corefers with. In other words, we should mark each document node with the labels of all summary nodes that refer to \purple{the same instance of the same concept}. To clarify, if there are multiple instances of the same concept - for example, if we had a dog named Roscoe and a dog named Nina in our example - we would only want to align \purple{matching instances} of the concept ``dog", so a dog node that corresponded to Roscoe in a document sentence would only get matched with the dog nodes corresponding to Roscoe in the summary sentences.\\

But there aren't any of these in our current example anyway; so for our example, we'd get something like this:

\begin{figure}[H]
    \centering
        \resizebox{0.5\textwidth}{!}{
    \includegraphics[height=4.5in]{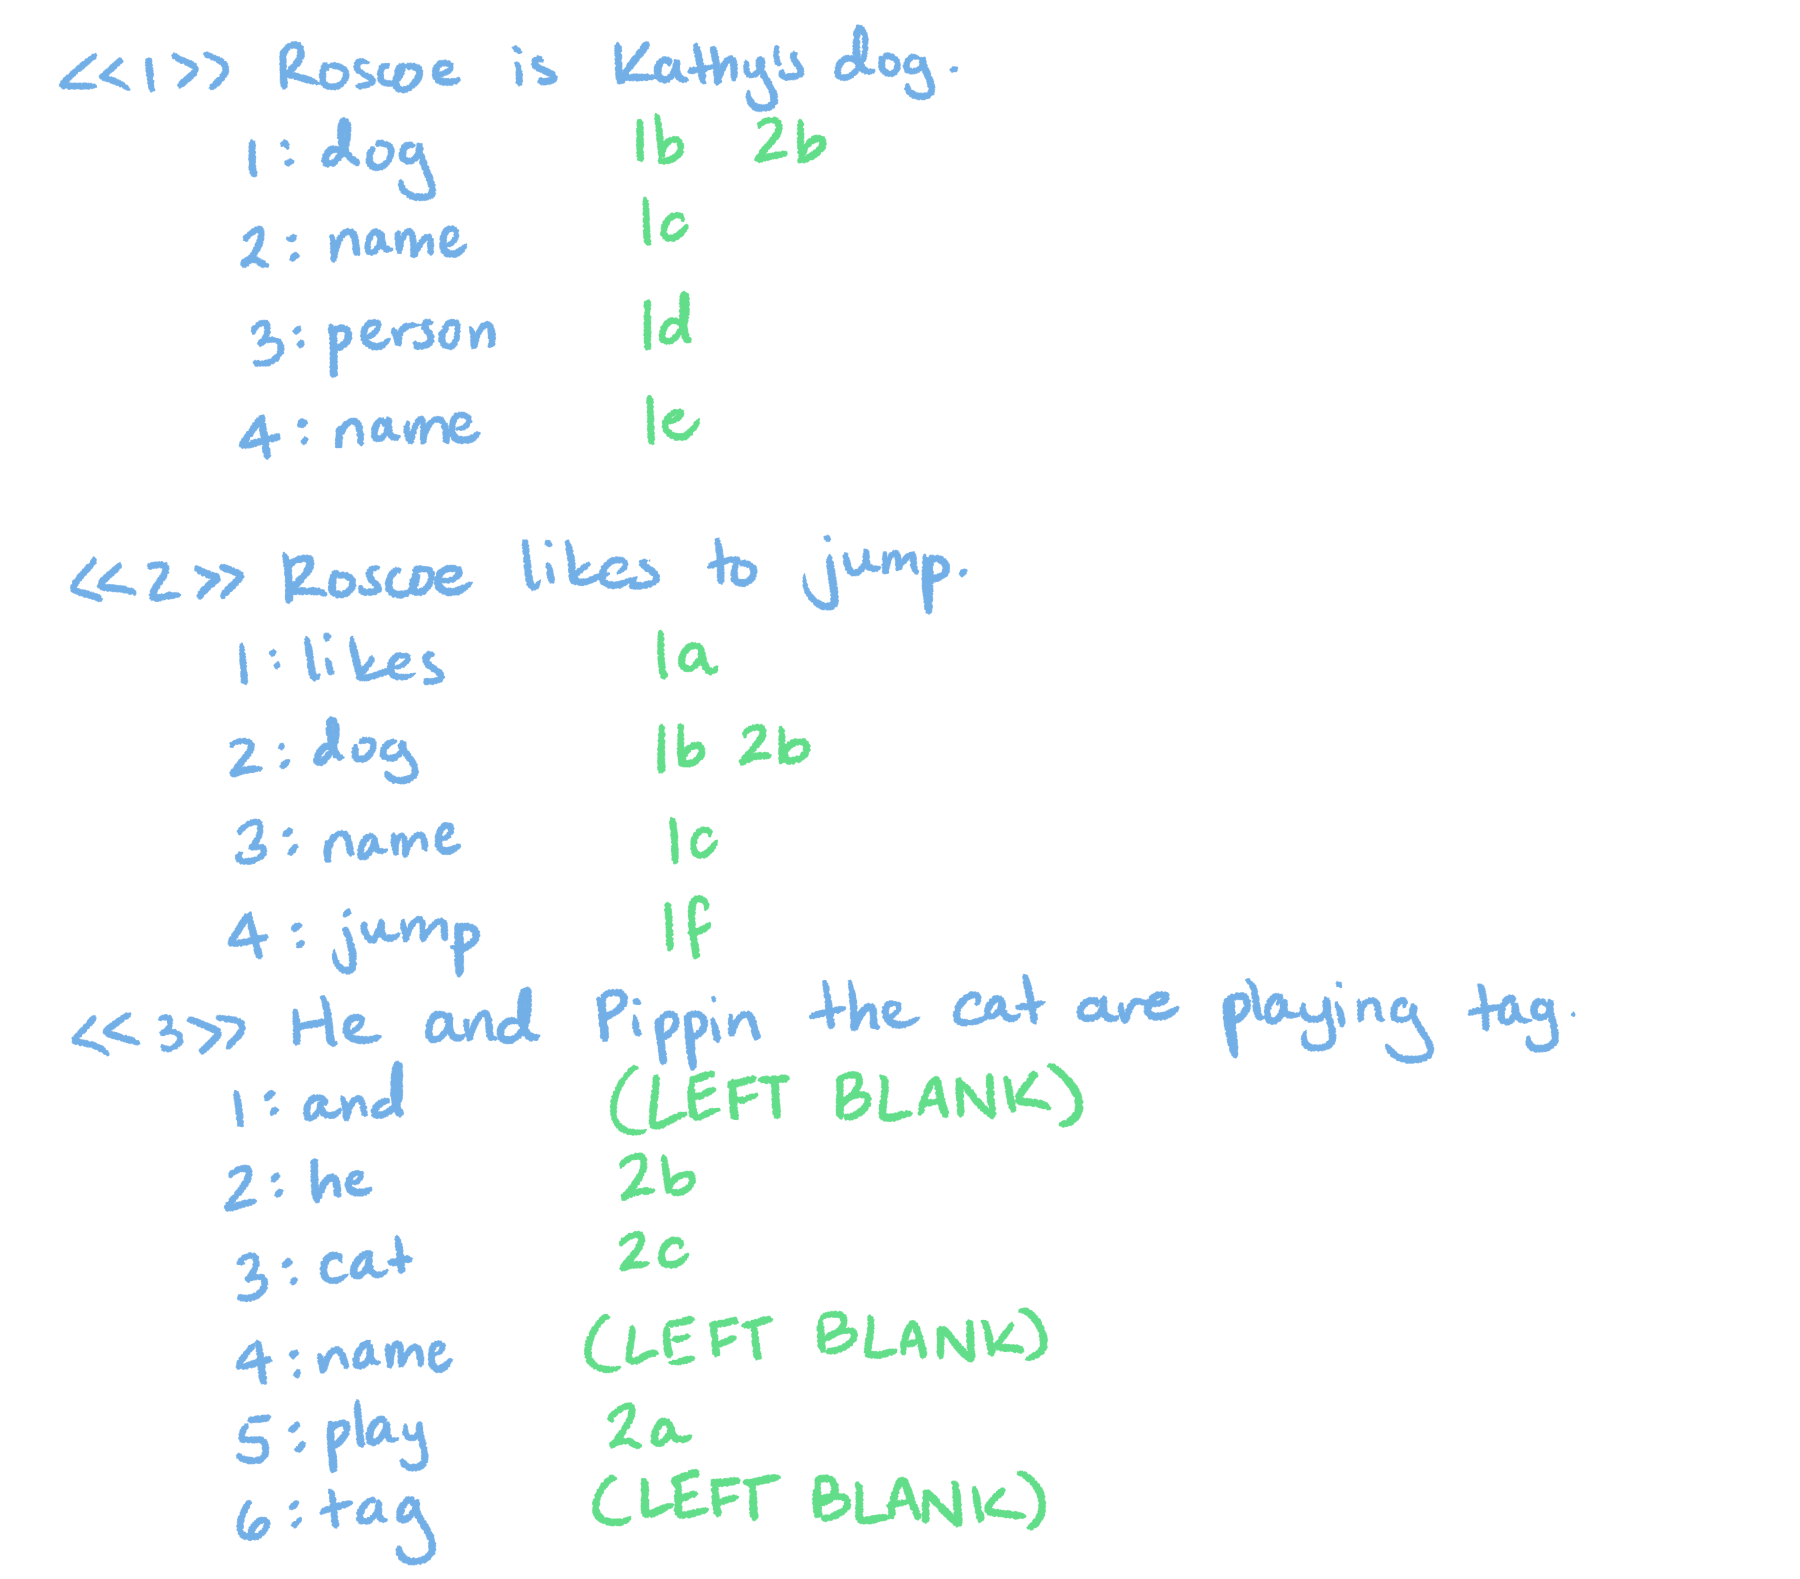}}
    \label{fig:sample-aligned}
\end{figure}

Note that the annotations for entities for which there is no match in the summary - ``and", Pippin's name, ``tag" - are \purple{not filled in}. I wrote ``(LEFT BLANK)" in the example so you can see the spaces, but you should leave them actually blank when you do the task.\\

Okay! Familiar with the basic structure of the task? Then let's dive into the real thing.

\paragraph{File format}
Each of the directories in this folder contains the files for a single document; the name of the folder is the document ID. Please mark your annotations in the main annotation file, \texttt{annotations.tsv}, and use the other files as reference. An example of a filled-out annotation file is provided in the \texttt{example/} directory.\\

\purple{Note on formatting: The annotation file is a tab-separated document. Please open it in some format that will allow you to keep track of the tab columns (e.g. as a spreadsheet).}\\

You are given a small number of sentences as reference at the top of the file that together form the summary for a single news document. Each sentence is followed by a list of corresponding ``entities" or nodes in the sentence's AMR graph, each indexed by a letter and the sentence number for each sentence. \purple{This was not programmatically enforced, but as a purely observational guideline, nodes tend to be listed in order of depth-first search over the AMR.}\\

Beneath the summary sentences is a series of sentences from the body of the original document. Each sentence is again followed by a list of entities that appear in the sentence, numbered separately for each document sentence. Once again, nodes are usually listed in depth-first order.\\

In case it's not clear from the text alone which part of a sentence an entity corresponds to, you are provided a number of extra files in the same directory as reference to disambiguate. The files provided as reference are the following: (1) an HTML file that visualizes \purple{text-to-node alignments}; and (2) one .png file for each document or summary sentence that contains a visualization of the AMR graph for that sentence.\\

In the alignments file, the summary sentences are in the floating blue box at the top and document sentences are beneath. \purple{Please note that these alignments are automatically generated, not hand-labeled, and they may be noisy; you should think of them more as hints as to what parts of the sentence each node corresponds to than as real guidelines.} If you use it, I would recommend opening the alignments file in a browser window and keeping it open side by side with the annotation file.\\

The graph visualizations look much the same as the sample graphs in the example we did above. If you find looking at graphs easier than reading node alignments, you're welcome to use those as reference instead.

\paragraph{Annotation instructions}
Please annotate each document sentence in \texttt{annotations.tsv} as follows: in the column immediately following each entity label, mark the identifier of the summary node that represents the \purple{same entity} (e.g. ``2a"). If there is no such summary node, leave this column blank. If there are multiple such nodes, \purple{write them all in a space-separated list in the same column} (e.g. ``1d 2c 3a").\\

If the document node is a descriptor or part of a descriptor and there is a summary node representing a similar descriptor, \purple{you should match them only if the nodes refer to the same instance of description}. For example, if we have a yellow dog in the document, and the same yellow dog as well as a yellow cat in the summary, the dog's ``yellow" in the document should only be matched to the dog's ``yellow" in the summary.\\

If there is no summary node that represents the same entity, but there is a summary node that represents \purple{an abstraction of that entity}, mark the identifier of that summary node in the first column after the entity label and write ``abs" in the second column. Some of the forms of abstraction you encounter may include:\\
\begin{itemize}
    \item Aggregation: e.g., the document nodes ``France", ``Germany" and ``Spain" all correspond to the summary node ``(European) countries".
    \item Generalization: e.g., the document node is labeled ``drives" but the summary node is labeled ``travels".
    \item Other: any other case where the document and summary nodes refer to the same concept but their meanings don't exactly match, e.g., the document node is ``organizes" but the summary node is ``funds".
\end{itemize}

However, note that even if two matching nodes have different labels, \purple{if they refer to the same object instance, the match should not be marked as abstractive.} For example, let's say Kathy is represented in the document by a ``person" node, and in the summary by an ``owner" node (of Roscoe) - in this case the two nodes should be matched without an abstractive label.

\paragraph{Annotation hints!}
I tried to break it down as clearly as possible in the example, but I know AMR is a kind of tricky format and can be hard to get used to. To help with this, you're given a lot of supporting reference materials in the annotation folders, but the sheer quantity of stuff to look at may make things confusing, especially for the first few annotations you do. Actually, as it turns out, most of the time you won't actually need to look at the reference files at all to do the task.\\

In this section I'll walk you through my approach to doing this annotation task in (what is for me) the quickest and most painless way. These aren't rules you have to follow, and if you find a different approach easier or more intuitive, you're welcome to do it your own way - but if you're a bit overwhelmed and are having trouble keeping track of all the information, this might be a useful guide.\\

Essentially, at the highest level, you want to do the following: (1) read the whole summary; (2) go through the document sentence by sentence, and go through each sentence entity by entity, and match each entity to the entities from the summary.\\

In the simplest possible steps, after reading the summary, for every document sentence, you want to:
\begin{enumerate}
    \item Read the sentence text.
    \item For the first entity, look at the label, then check if the entity makes an appearance in each summary sentence; if it does, look for the corresponding entity identifier and mark it down (or add it to the list of marked identifiers).
    \item For the second entity, do the same thing.
    \item Do it again for the third entity.
    \item Etc.
\end{enumerate}

That may sound really dry and repetitive, but it's actually a lot quicker than it seems - most of the time you can figure out if an entity appears in a summary sentence nearly instantaneously by looking back at the sentence text, and finding the identifier just means going through the list of node labels and picking the right one.\\

To make this a little more concrete, let's go back to our original example. First we'll read the summary: \green{Kathy's dog Roscoe likes to jump. He is playing with a cat.} And here's our summary node list:

\begin{figure}[H]
    \centering
            \resizebox{0.5\textwidth}{!}{
    \includegraphics{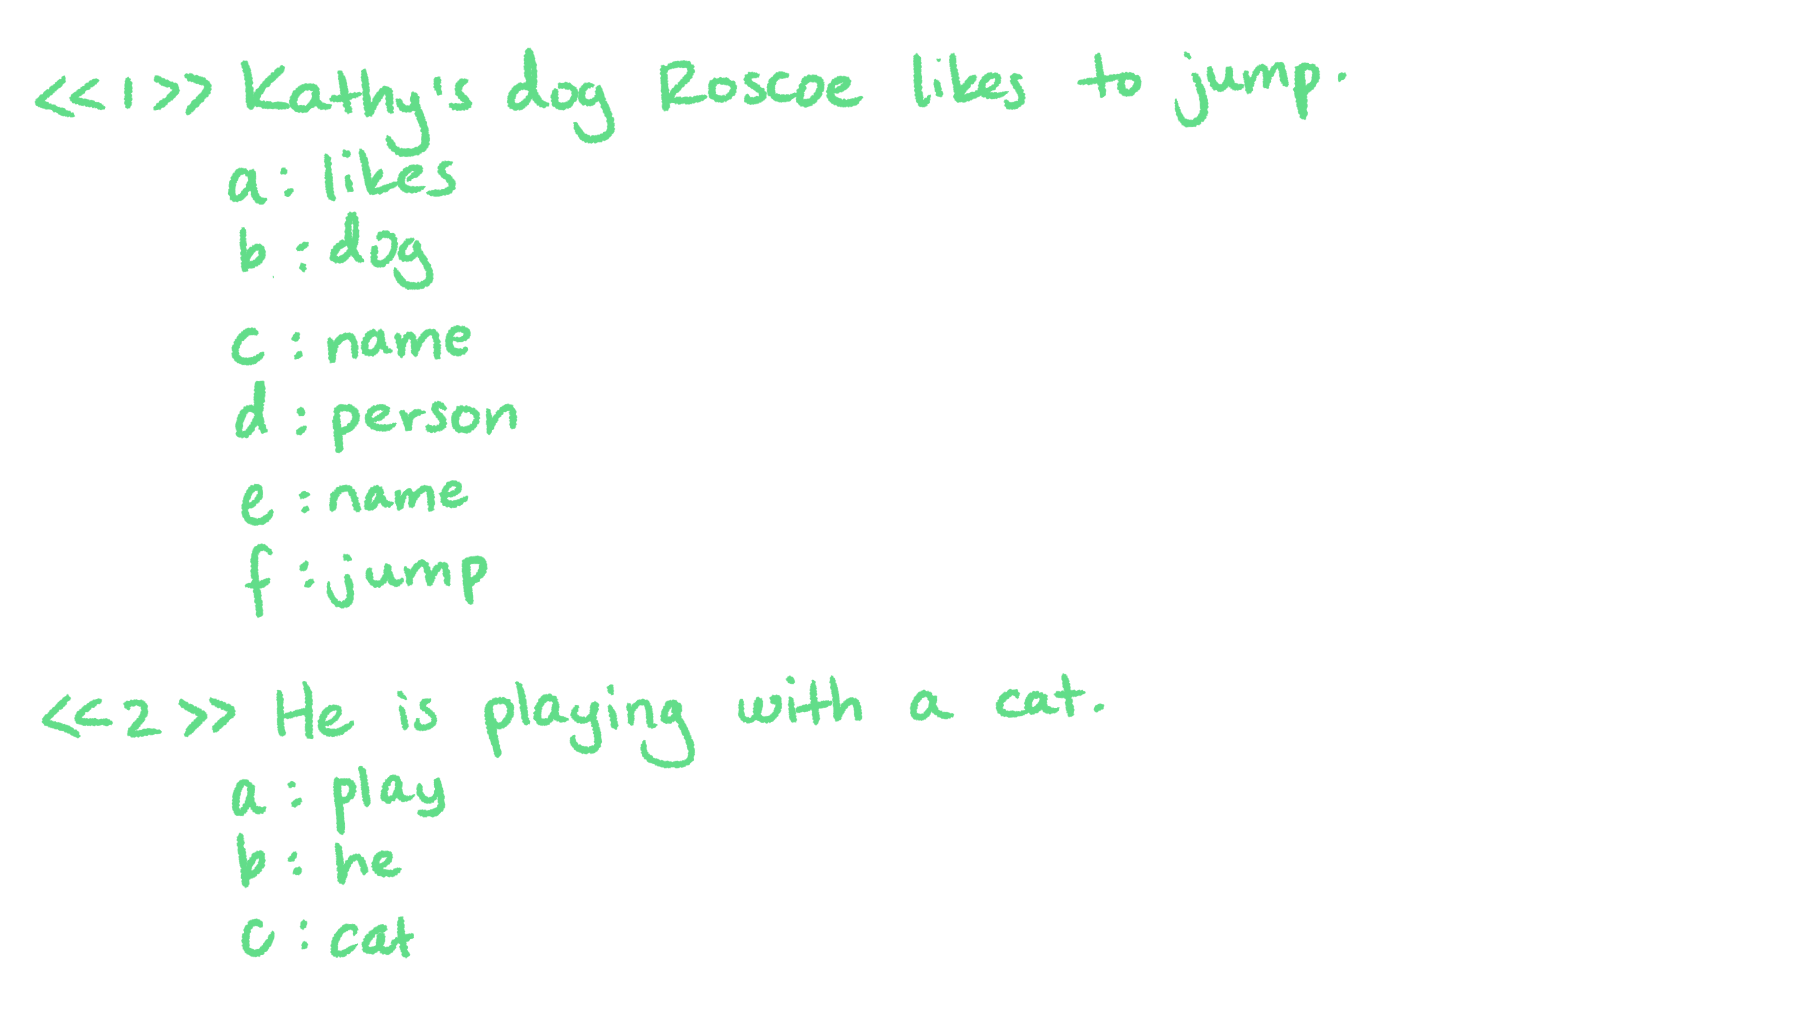}
    }
    \label{sample-summary-nodes}
\end{figure}

Alright, cool. Let's look at our first document sentence.

\begin{figure}[H]
    \centering
            \resizebox{0.5\textwidth}{!}{
    \includegraphics{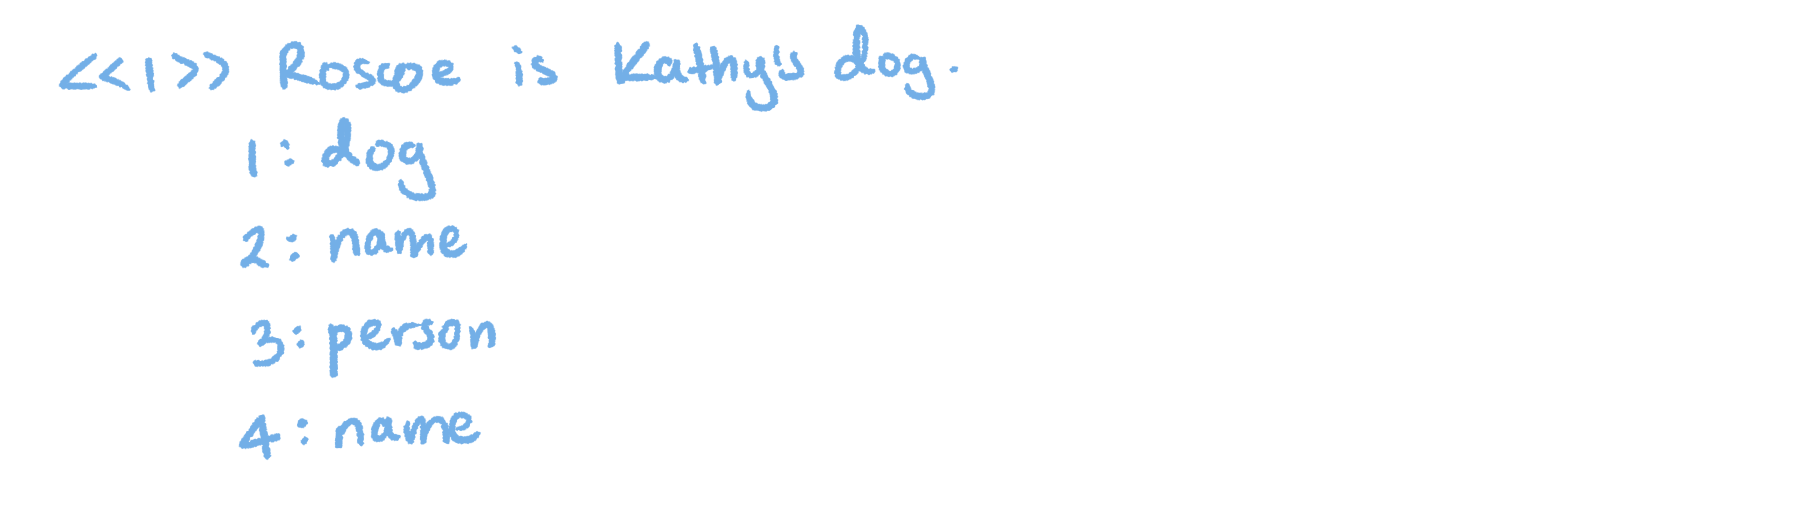}
    }
    \label{sample-single}
\end{figure}

The sentence is \blue{Roscoe is Kathy's dog.} Great. The first entity is labeled \blue{1: dog}. Well, there's only one dog in this sentence, so we know what dog this is, it's Roscoe. Alright, now let's go back to our summary sentences. Is Roscoe in the first sentence? Yes he is! And which entity corresponds to our \blue{1: dog}? Looks like \green{1b: dog}. So we'll write down \green{1b}. Now the second summary sentence, ``\green{He is playing with a cat}." Is Roscoe in this sentence? Yup, he's here too. In this case there's no \texttt{dog} node, but the node \green{2b: he} corresponds to the same entity, so we'll also mark down \green{2b}.\\

That's all the summary sentences, so our complete annotation for \blue{1: dog} is \green{1b 2b}.\\

Now we can move on to the next node, \blue{2: name}. Once again - is Roscoe's name in the first sentence? Yup, \green{1c: name}. Is it mentioned in the second sentence? No. So the annotation for \blue{2: name} is \green{1c}. And we can go on similarly for the rest of the entities.\\

I wrote it out in a rather long-winded way, but, again, these judgements don't take very long in practice. There are some additional timesaving tricks you'll probably notice when you do the task, too. For example, \purple{nodes are often listed in a consistent order}, so you'll sometimes get multiple nodes in a row that correspond exactly to another list of multiple nodes in a row in a summary sentence. Another thing that can save time, if you really dislike scrolling, is actually just \purple{rereading your annotations} from the previous document sentence - if you notice any nodes in common between the sentence you're currently looking at and the previous one, you can just copy in the annotations you already did for that entity in the previous sentence :)\\

One more thing to note when looking at the real annotations is that some nodes may have slightly confusing labels - a good example is the common \texttt{have-org-role-91}, which does basically what it says on the tin (indicates a relationship of belonging to an organization), but may be hard to interpret at first glance. \purple{If you're not sure what a node does, check its position in the graph.}\\

You'll probably come up with your own shortcuts and find your own annotation style as you go. Hopefully all this explication didn't scare you off! Once again, thanks so much for agreeing to do these annotations, and good luck on the task!

\paragraph{Longer example}
Okay, so we walked through a pretty baby example in section 4. The real sentences are a little more complicated than that. In this section we'll go through the first few sentences of the example annotation file included in the \texttt{example/} directory.\\

Once again, our first step is to read the entire summary. In this case it's only one sentence.
\begin{figure}[H]
    \centering
                \resizebox{0.5\textwidth}{!}{
    \includegraphics[width=7in]{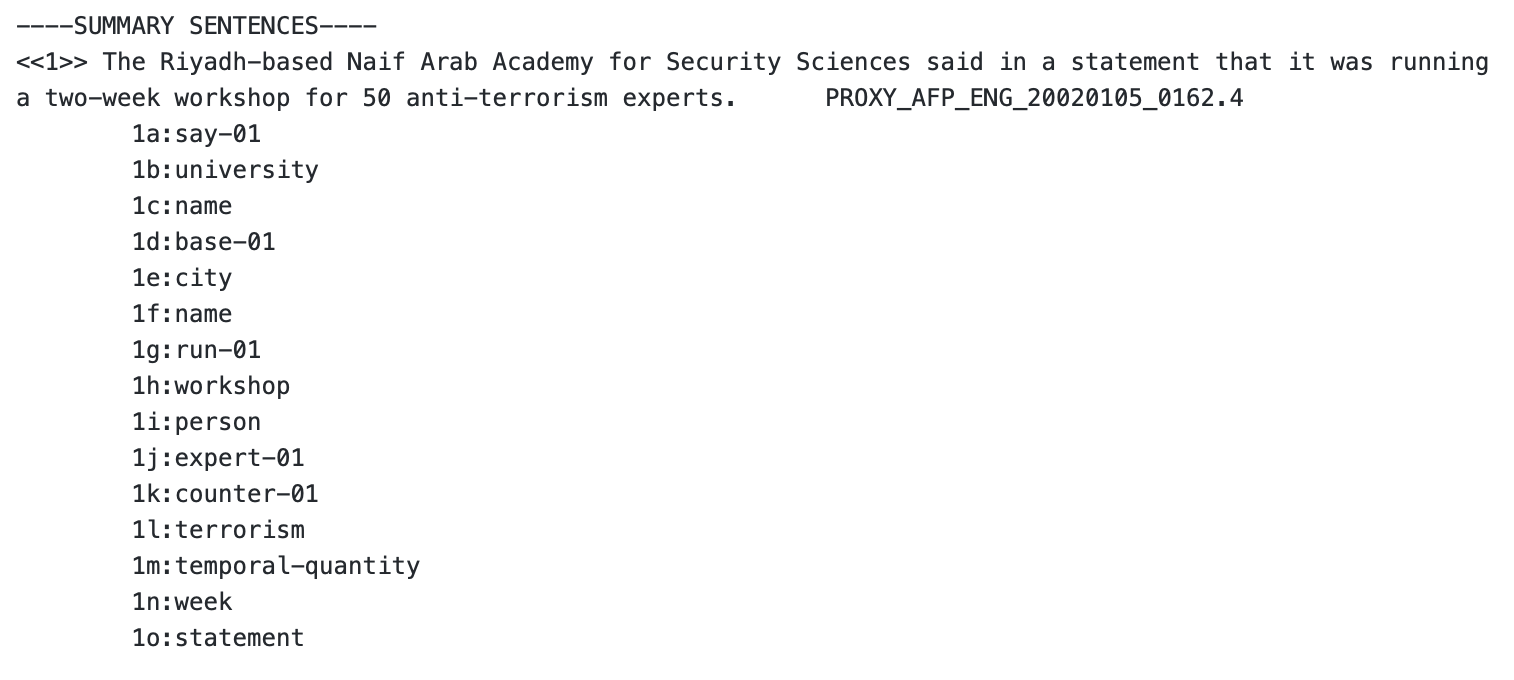}}
    \label{fig:long-summary}
\end{figure}

Okay. So we read our summary; now on to the main document.
\begin{figure}[H]
    \centering
                    \resizebox{0.5\textwidth}{!}{
    \includegraphics[width=7in]{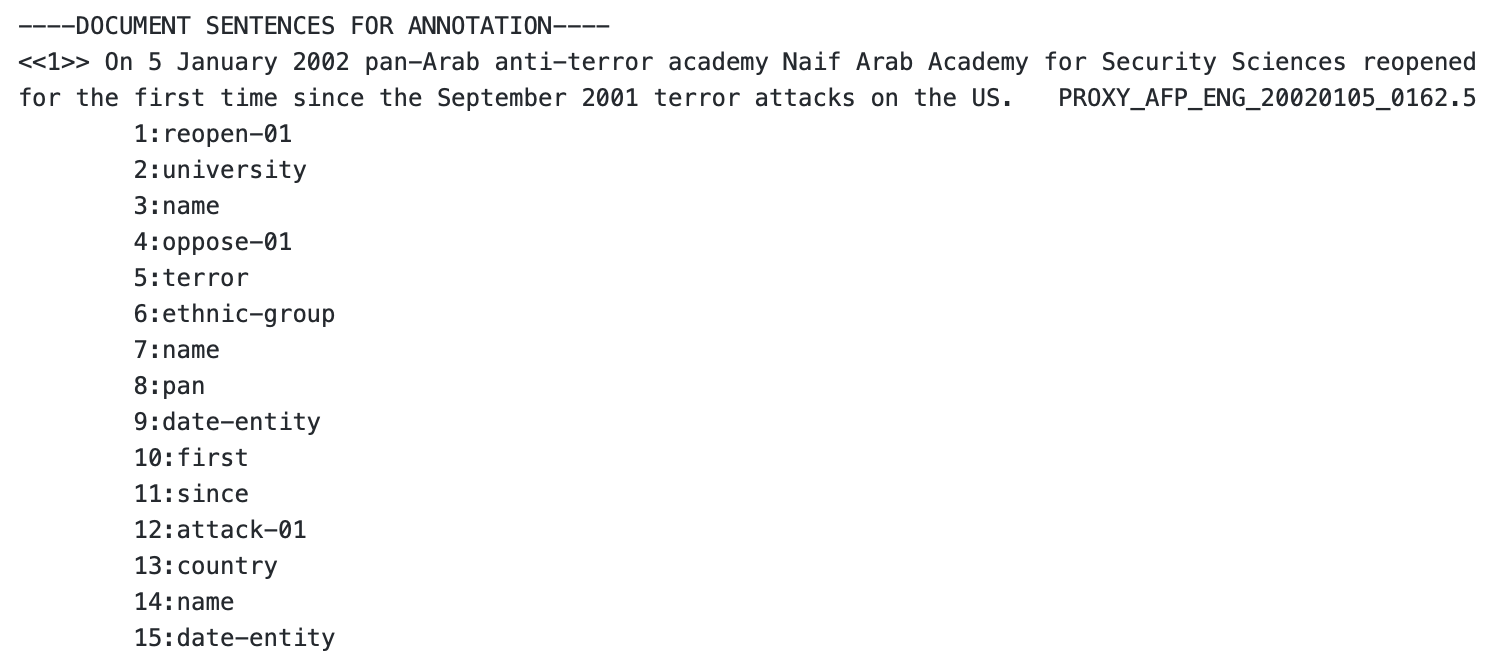}}
    \label{fig:long-document-1}
\end{figure}

We'll start off with the first sentence. Again, first we'll read the text to get a sense for what's going on.\\

Next we'll start going through the entities. \blue{1:reopen-01} obviously corresponds to the academy reopening in the sentence; does this occur in the summary? Nope, no reopening there. Skip. \blue{2:university} must refer to the academy; does this occur in the summary? Yes, and there it's represented by the node \green{1b}. How about \blue{3:name}? We don't actually know just from looking at the label which name this node corresponds to, but if the entity ordering here is depth-first, we can make a pretty good guess that it's attached to the \blue{2:university} node.\\

(If we open up the graph visualization for this sentence we can confirm this:)
\begin{figure}[H]
    \centering
    \resizebox{0.45\textwidth}{!}{
    \includegraphics{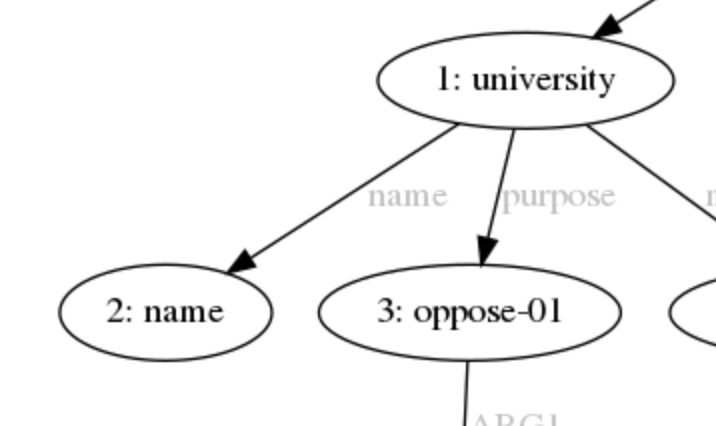}}
    \label{fig:long-graph-1}
\end{figure}

Okay, so it's the name of the academy. Does this name appear in the summary? Yes, it's node \green{1c}. Alright, how about \blue{4:oppose-01}? Since it's attached to the university, seems like it's the ``anti" in ``anti-terror". Does this appear in the summary? This is actually a \purple{slightly tricky case} - there's no ``anti-terror" descriptor in the summary, but there is an ``anti-terrorism". So we have to decide whether the anti-terror here corresponds with the anti-terrorism in the summary. It could be argued for either way, but for consistency we need to pick a rule of thumb, and our rule of thumb is that we only want to match a descriptor with the same instance of description. In this case ``anti-terror" is used to describe something different in ``anti-terror academy" and in ``anti-terrorism experts"; so we're going to say \purple{no}.\\

Same goes for \blue{5:terror}; this is part of the same descriptive phrase. Then next, how about \blue{6:ethnic-group}? This refers to ``Arab" in ``pan-Arab". Then is there an ``Arab" in the summary? This is \purple{another slightly tricky case} - there is an ``Arab", but it's used in the context of a name, ``Naif Arab Academy for Security Sciences". Just from the rule we used above, we can say that these two shouldn't get matched, since ``pan-Arab" is definitely a different descriptor than ``Arab" in ``Arab Academy"; but something specific to note is that since ``Arab" is used as part of the academy's name, \purple{we don't actually want to count it as a descriptor at all} in that usage. Rather, it's more useful to consider it being used as a special token that only takes on its meaning in that particular context. In practice, the tokens in the name of the academy won't actually show up in the AMR at all, so we don't have to worry about matching things to the individual words. Just don't decide to match anything else to the name node because of the tokens in it! In this case, our \blue{6:ethnic-group} stays unmatched.\\

Next up is \blue{7:name}, which presumably refers to ``Arab". Again, no match. Then \blue{8:pan}, which is obvious, and again is unmatched. \blue{9:date-entity} probably refers to the first date in the sentence, which we can confirm with the graph; no dates in the summary, so no match. None of the information from the whole clause ``for the first time since the September 2001 terror attacks on the US" appears in the summary, so \blue{10:first}, \blue{11:since}, \blue{12:attack-01}, \blue{13:country}, \blue{14:name} and \blue{15:date-entity} are all unmatched.\\

Phew. Okay, we're done with the first sentence. Thankfully, the next one is a lot easier.
\begin{figure}[H]
    \centering
\resizebox{0.5\textwidth}{!}{
    \includegraphics[width=7in]{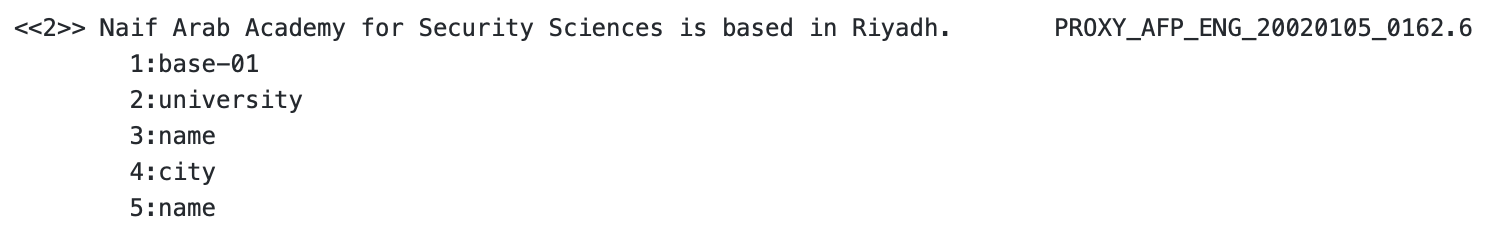}}
    \label{fig:long-document-2}
\end{figure}

Read the sentence. Okay, \blue{1:base-01}? Yep, it corresponds exactly to \green{1d}. Actually, the rest of the nodes have a one-to-one correspondence with nodes from the summary as well - \blue{2:university} is \green{1b}, \blue{3:name} is \green{1c}, \blue{4:city} is \green{1e}, and \blue{5:name} is \green{1f}. Easy.\\

Alright, next the third sentence.
\begin{figure}[H]
    \centering
    \resizebox{0.5\textwidth}{!}{
    \includegraphics[width=7in]{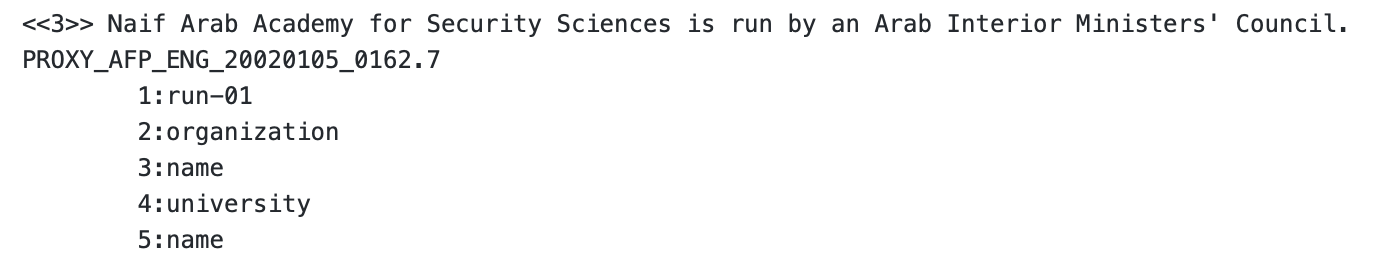}}
    \label{fig:long-document-3}
\end{figure}

This one isn't too bad either - as long as we're a little careful. Our first entity is \blue{1:run-01}, and we might be immediately tempted to say, ah, this must match the summary node \green{1g:run-01}. This is why it's important to read the sentence first! In this case, the Arab Interior Ministers' Council is \textit{running the academy}; in the summary, \textit{the academy} is running the workshop. So these are actually two different instances of the same verb, ``run-01". So no match here.\\

The other nodes aren't too bad. \blue{2:organization} and \blue{3:name} refer to the Ministers' Council, which doesn't appear in the summary for either; \blue{4:university} and \blue{5:name} refer to our good friend Naif Arab Academy for Security Sciences, and we can actually take a shortcut here and rather than scrolling all the way back up to the summary, just look back at our previous sentence for the annotations. What did we write? The \blue{university} node for the academy gets matched to \green{1b}, and the \blue{name} node gets matched to \green{1c}. Cool, we can just copy that in.\\

And we're done with the first three sentences. The rest of the document goes much the same way. Again, I kind of expanded this out as much as possible, but in reality you'll just be thinking all of this to yourself relatively quickly, so don't be daunted! It's a lot faster than it reads.
